# Supplementary material for: Efficient Simulation of Loop Quantum Gravity -- A Scalable Linear-Optical Approach
Source: arXiv:2003.03414 ancillary file (2021-01-03)
Supplement: Supplementary file 1 [file linear_optical_LQG__supplementary_material.pdf]

# Supplementary Material: "Simulation of Loop Quantum Gravity — A Scalable Linear-Optical Approach"

Lior Cohen,[1] Anthony J. Brady,[1] Zichang Huang,[2,3] Hongguang Liu,[4] Dongxue Qu,[5] Jonathan P. Dowling,[1,6,7,8] and Muxin Han[5,9]

[1]*Hearne Institute for Theoretical Physics, and Department of Physics and Astronomy, Louisiana State University, Baton Rouge, Louisiana 70803, USA.*
[2]*Department of Physics, Center for Field Theory and Particle Physics, and Institute for Nano- electronic devices and Quantum computing, Fudan University, Shanghai 200433, China*
[3]*State Key Laboratory of Surface Physics, Fudan University, Shanghai 200433, China*
[4]*Center for Quantum Computing, Pengcheng Laboratory, Shenzhen 518066, China*
[5]*Department of Physics, Florida Atlantic University, 777 Glades Road, Boca Raton, FL 33431, USA*
[6]*NYU-ECNU Institute of Physics at NYU Shanghai, 3663 Zhongshan Road North, Shanghai, 200062, China.*
[7]*CAS-Alibaba Quantum Computing Laboratory, CAS Center for Excellence in Quantum Information and Quantum Physics, University of Science and Technology of China, Shanghai 201315, China.*
[8]*National Institute of Information and Communications Technology, 4-2-1, Nukui-Kitamachi, Koganei, Tokyo 184-8795, Japan*
[9]*Institut für Quantengravitation, Universität Erlangen-Nürnberg, Staudtstr. 7/B2, 91058 Erlangen, Germany*

We show, in details, how the unitary transformation can be decomposed into linear optics elements, including a numerical example and the Matlab code used. In addition, more details about the Von Neumann entropy are presented.

## From unitary transformation to linear optics

Here we show how $U$ can be reconstructed by series of two-mode unitary operations where the other modes remain unchanged [1, 2]. Each operation consists with two 50:50 beamsplitters and two phase shifters, which are implementable with linear optics [1]. Configuring these elements in a Mach-Zehnder interferometer (MZI) with a phase shifter at one output port results in the following transformation:

$$T'_{\mathrm{MZI}}(\phi,\omega)=\begin{pmatrix} e^{i\phi}\sin\omega & e^{i\phi}\cos\omega \\ \cos\omega & -\sin\omega \end{pmatrix}, \tag{S1}$$

where $\omega$ is the phase inside the MZI and $\phi$ is the phase after the MZI. The MZI transformation is equal to a beamsplitter with arbitrary transmission and phase.

Since $U$ is unitary, its rows and columns form an orthonormal basis. Thus, each row and column has a size of one. We reconstruct $U$ by transforming it into the identity matrix $I$. We start by transforming the last raw of $U$ to the trivial basis vector:

$$\begin{pmatrix} U(N,1) \\ U(N,2) \\ \vdots \\ U(N,N) \end{pmatrix}^T \xrightarrow{T_N} \begin{pmatrix} 0 \\ 0 \\ \vdots \\ 1 \end{pmatrix}^T, \tag{S2}$$

where the indices inside the parenthesis are the matrix-element coordinates, while subscripts indicate the row(s) which the $2\times 2$ transformation is applied on. For every $j=1,\ldots,N-1$, $U(N,j)$ can be independently set to zero by multiplying from the right by $T'_{N,j}$ of Eq. S1 with $\phi=\arg(U(N,N)/U(N,j))+\pi$, $\omega=\tan^{-1}(|U(N,N)/U_(N,j)|)$, and the argument function returns the phase of a complex number. From the $2\times 2$ matrix, $T'_{N,j}$, an $N\times N$ matrix, $T_{N,j}$, is built by taking the identity matrix and replacing the elements of the intersections of the $j,N$ rows and columns by the $T'_{N,j}$ elements:

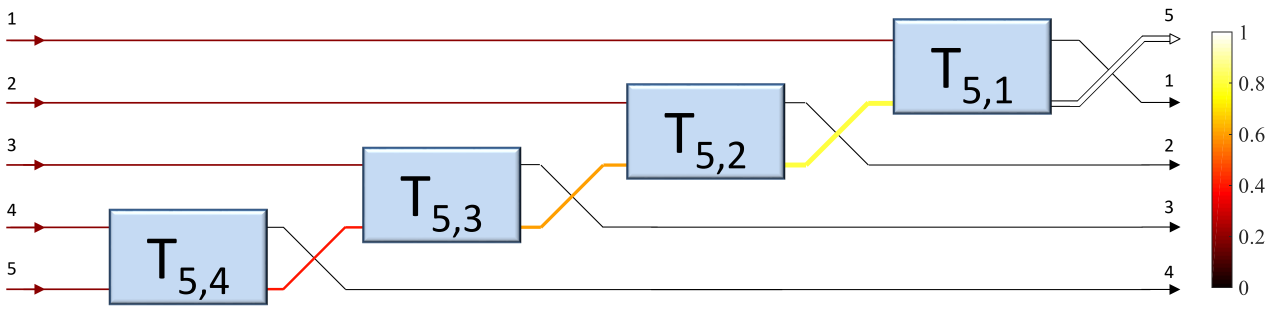


FIG. 1: Illustration of Eq. S2 for five modes. In this illustration, all modes are initially occupied symmetrically. Step by step, all the elements of the five-vector are set to zero as described in the text. At the end, there is only one non-zero element, as in the R.H.S. of Eq. S2. The color and the width of the lines correspond to the value of the mode, where darker and thinner indicate lower values.

$$T_{N,j} = \begin{array}{c} \\ \left( \begin{array}{ccccc} 1 & 0 & \cdots & & 0 \\ 0 & \ddots & & & \\ \vdots & & 1 & & \\ & & & T'_{N,j}(1,1) & T'_{N,j}(1,2) \\ 0 & & & T'_{N,j}(2,1) & T'_{N,j}(2,2) \end{array} \right) \end{array} \begin{array}{c} \\ \\ \\ j \\ N \end{array} \tag{S3}$$

(column labels above the matrix: $j$, $N$)

After $N-1$ transformations, the last row becomes the trivial basis vector of Eq. S2 up to a phase, $T_N = T_{N,N-1} \cdot T_{N,N-2} \cdot \ldots \cdot T_{N,1}$. Since only unitary matrices were multiplied, the outcome is also unitary, thus the last column has only one non-zero element, and the new matrix is

$$\left( \begin{array}{cc} \left[ \quad U' \quad \right] & \begin{array}{c} 0 \\ 0 \\ \vdots \\ 0 \end{array} \\ 0 \;\; 0 \;\; \cdots \;\; 0 & e^{i\alpha_N} \end{array} \right), \tag{S4}$$

where $U'$ is another $(N-1) \times (N-1)$ unitary matrix and $\alpha_N$ is some phase. By induction, $U$ can be inverted, i.e. $U \cdot T_{N,N-1} \cdots T_{N,1} \cdot T_{N-1,N-2} \cdots T_{N-1,1} \cdots T_{2,1} \cdot D = I$, where $D$ is diagonal matrix compensating for the phases. Since $U$ is unitary, we may reconstruct it with only linear optics transformations:

$$U = D^{\dagger} \cdot T_{2,1}^{\dagger} \cdots T_{N,N-1}^{\dagger} \,. \tag{S5}$$

**Example**

We now show an example of the described procedure for a particular gate A, given by the spinfoam vertex amplitude

$$A = \begin{pmatrix} 0.426 & -0.003 & 0.003 & -12.3 & 0 & 0.0286 & 0.0286 & 0 \\ 0 & -0.004 & -0.004 & 0 & -0.035 & 0.429 & -0.429 & 29.2 \\ 0 & -0.006 & -0.006 & 0 & 0.009 & -40.8 & 40.8 & 24.4 \\ -11.9 & -0.038 & 0.038 & 290 & 0 & 24.8 & 24.8 & 0 \end{pmatrix} \times 10^{-9} \tag{S6}$$

For display purposes, we keep only the three significant digits. $A$ is obtained numerically from the vertex amplitude of Engle-Pereira-Rovelli-Livine (EPRL) spinfoam model when all spins $j = 2$ and Barbero-Immirzi parameter $\gamma = 1.2$. A choice of the 2D subspace $\mathcal{H}_{\text{tet}}^{(2D)} \subset \mathcal{H}_{\text{tet}}$ is made since the space $\mathcal{H}_{\text{tet}}$ of quantum tetrahedra has dimension higher than two. The numerical computation uses the technique in Ref. [3]. The singular values of A are $\begin{pmatrix} 292 & 80.9 & 37.9 & 1.52 \end{pmatrix} \times 10^-9$ which is less than one. All the other matrices we checked, produced in the same way with different values of $j$ and $\gamma$, also have singular values less than one. This satisfies the condition for extending A to a unitary matrix.

After decomposing A to its singular values and extending A to a unitary matrix U (as described in the main text), we decompose U (up to single-mode phases, corrected by the matrix D) to the linear-optical transformations as in Eq. S5:

$$U = \prod_{i=2}^{12} \prod_{j=1}^{i-1} T'_{\text{MZI}}(\phi(i,j), \omega(i,j))^\dagger\,, \tag{S7}$$

where $\phi(i,j)$ ($\omega(i,j)$) are the inside and outside phases of the interferometer between the $i^{\text{th}}$ and $j^{\text{th}}$ spatial modes. We plot the matrices of phases for the example A (Eq. S6):

$$\phi = \begin{pmatrix} 0 & 0 & 0 & 0 & 0 & 0 & 0 & 0 & 0 & 0 & 0 & 0 \\ 1.1 & 0 & 0 & 0 & 0 & 0 & 0 & 0 & 0 & 0 & 0 & 0 \\ 0.1 & 0 & 0 & 0 & 0 & 0 & 0 & 0 & 0 & 0 & 0 & 0 \\ 0.2 & 0.2 & 0.2 & 0 & 0 & 0 & 0 & 0 & 0 & 0 & 0 & 0 \\ 1 & 0 & 1 & 1 & 0 & 0 & 0 & 0 & 0 & 0 & 0 & 0 \\ 1 & 0 & 0 & 1 & 0 & 0 & 0 & 0 & 0 & 0 & 0 & 0 \\ 1 & 1 & 0 & 0 & 1 & 0 & 0 & 0 & 0 & 0 & 0 & 0 \\ 0 & 0 & 1 & 0 & 0 & 1 & 0 & 0 & 0 & 0 & 0 & 0 \\ 1 & 1 & 1 & 0 & 0 & 0 & 0 & 1 & 0 & 0 & 0 & 0 \\ 1 & 0 & 0 & 1 & 0 & 0 & 0 & 0 & 1 & 0 & 0 & 0 \\ 0 & 1 & 0 & 1 & 1 & 0 & 0 & 1 & 1 & 0 & 0 & 0 \\ 0 & 1 & 1 & 0 & 0 & 0 & 0 & 0 & 1 & 1 & 0 & 0 \end{pmatrix} \times \pi \tag{S8}$$

$$\omega = \begin{pmatrix} 0 & 0 & 0 & 0 & 0 & 0 & 0 & 0 & 0 & 0 & 0 & 0 \\ 0.5 & 0 & 0 & 0 & 0 & 0 & 0 & 0 & 0 & 0 & 0 & 0 \\ 0.5 & 0.187 & 0 & 0 & 0 & 0 & 0 & 0 & 0 & 0 & 0 & 0 \\ 0.011 & 0.315 & 0 & 0 & 0 & 0 & 0 & 0 & 0 & 0 & 0 & 0 \\ 0 & 0.013 & 0.185 & 0 & 0 & 0 & 0 & 0 & 0 & 0 & 0 & 0 \\ 0.493 & 0 & 0.039 & 0.055 & 0.482 & 0 & 0 & 0 & 0 & 0 & 0 & 0 \\ 0.497 & 0.363 & 0 & 0.029 & 0.399 & 0.049 & 0 & 0 & 0 & 0 & 0 & 0 \\ 0.054 & 0.496 & 0.496 & 0 & 0.499 & 0.4 & 0.8 & 0 & 0 & 0 & 0 & 0 \\ 0.5 & 0.5 & 0.5 & 0.5 & 0 & 0.492 & 0.169 & 0 & 0 & 0 & 0 & 0 \\ 0.496 & 0.5 & 0.5 & 0.04 & 0.5 & 0 & 0.101 & 0.248 & 0.497 & 0 & 0 & 0 \\ 0.498 & 0.5 & 0.5 & 0.25 & 0.5 & 0.293 & 0 & 0.435 & 0.487 & 0.434 & 0 & 0 \\ 0.5 & 0.5 & 0.5 & 0.5 & 0.5 & 0.405 & 0.4 & 0 & 0.5 & 0.481 & 0.2 & 0 \end{pmatrix} \times \pi \tag{S9}$$

The triangular shape of the matrices is a result of interfering two modes only once and not interfering the mode with itself. Notice that the $\omega$ matrix has 11 zeros which means, for this gate A, only 55 MZI are needed.

In additional to $A$ in Eq. (S6), we have also tested our program on other vertex amplitudes with different $j$ and $\gamma$, including ($j = 1/2,\ \gamma = 1.2$), ($j = 1/2,\ \gamma = 1$), ($j = 1/2,\ \gamma = 0.1$), and ($j = 1,\ \gamma = 1.2$). The code to generate these matrices is attached at the end of this supplementary material.

## Von Neumann entropy

In order to provide evidence that this is a true quantum simulation, we evaluate the amount of path entanglement in the output state. We calculate the Von Neumann entropy after the partial trace. There are 14 different ways to carry out a partial trace over four-spatial modes; four ways to trace over one mode, six ways to trace over two modes and four ways to trace over three modes. Here, we maximize over all possible traces to calculate the entropy.

For example, let us take A of Eq. S6, and the initial state of a single photon in the seventh mode. The normalized output state is $|\Psi\rangle_{out} = \sum_{n=0}^{3} \alpha_n |n\rangle$, where the amplitudes (after post selection) are

$$\begin{pmatrix} 0.000457 & -0.642 & 0.656 & 0.397 \end{pmatrix} . \tag{S10}$$

Tracing over one mode out of four gives the entropy:

$$\begin{pmatrix} 4.94 \times 10^{-6} & 0.978 & 0.986 & 0.629 \end{pmatrix} . \tag{S11}$$

Tracing over two modes out of four gives the entropy:

$$\begin{pmatrix} 0.978 & 0.986 & 0.629 & 0.629 & 0.986 & 0.978 \end{pmatrix} . \tag{S12}$$

The entropy while tracing over three modes is equal to the entropy of tracing over the fourth mode. Maximizing over all options, we get an entropy of 0.986. Inputting the photon into each of the eight spatial modes and repeating the same procedure, results in the entropy:

$$\begin{pmatrix} 0.014 & 0.227 & 0.227 & 0.019 & 0.358 & 0.986 & 0.986 & 0.977 \end{pmatrix} . \tag{S13}$$

This means the entanglement ranges between $0.014 - 0.986$ as stated in the main text.


[1] M. Reck, A. Zeilinger, H. J. Bernstein, and P. Bertani, Physical Review Letters **73**, 58 (1994).

[2] W. R. Clements, P. C. Humphreys, B. J. Metcalf, W. S. Kolthammer, and I. A. Walmsley, Optica **3**, 1460 (2016).

[3] P. Donà, M. Fanizza, G. Sarno, and S. Speziale, Phys. Rev. **D100**, 106003 (2019), 1903.12624.

## The matlab code

```
%% Finding the unitary
[L, S, R] = svd(A); % A = L*S*R' is the 4x8 gate matrix
% svd is matlab function.
U = [A, L*sqrt(eye(4)-S*S')*L; R'*sqrt(eye(8)-S'*S)*R', -
R'*S'*L];
% U is the unitary expansion of A, eye(n) is the n-row identity
% matrix and sqrt is a matlab fuction for square root
tmp1 = U'*U-eye(12); sum(abs(tmp1(:))) % checking the unitarity
%% setting parameters
U2 = U;
J1 = length(U2);
w1 = zeros(J1);
D = w1;
phi1 = w1;
%% decomposing the unitary to linear optics
for j = J1:-1:2 % running over rows
    for k = j-1:-1:1 % running over columns
        c = U2(j,k);
        if abs(c)>1e-15 % run only if larger than 1e-15
            d = U2(j,j);
            if abs(d)<1e-15
               % set the value to zero if smaller than 1e-15
                d=0;
            end
            phi1(j,k) = phase(d/c)+pi; % the value of the phases
            w1(j,k) = atan(abs(d/c));
               T = [exp(1i*phi1(j,k))*sin(w1(j,k)),...
               exp(1i*phi1(j,k))* cos(w1(j,k)); cos(w1(j,k)),...
               -sin(w1(j,k))];
            % the MZI transformation
            U1 = eye(J1);
               U1(k,k) = T(1,1);U1(j,j) = T(2,2);
               U1(k,j) = T(1,2); U1(j,k) = T(2,1);
            % make 12x12 matrix with the MZI transformation
            U2 = U2*U1;
        end
    end
end
for k=1:J1
    D(k,k) = exp(1i*phase(U2(k,k))); % the phase matrix
end
U2 = U2*D';
tmp1 = U2 - eye(12); sum(abs(tmp1(:)))
% checking we got the identity matrix
```
